# Supplementary material for: Hybrid Beam Alignment for Multi-Path Channels: A Group Testing Viewpoint
Source: arXiv:2111.08159 source file (2022-05-13)
Supplement: Supplementary file 1 [file qual_additional.tex]

\documentclass[conference,letter]{IEEEtran}
\IEEEoverridecommandlockouts

\usepackage{color}
\usepackage{amsthm}
\usepackage{mathtools}

\usepackage{bbm}
\usepackage{amssymb}
\usepackage{tikz}
\usepackage{comment}
\usepackage{enumitem}
\usepackage[ruled,vlined, linesnumbered]{algorithm2e}

\SetCommentSty{mycommfont}

\RestyleAlgo{ruled}
\SetInd{0em}{0.5em}
\SetKwComment{Comment}{/\!\!/}{}
\usepackage{booktabs}
\usepackage{cite}
\usepackage{steinmetz}
\usepackage{subcaption}
\usepackage{dblfloatfix}

\hyphenation{op-tical net-works semi-conduc-tor}

\usepackage{caption}
\captionsetup[table]{labelsep=period}

\input{others/com.tex}

\begin{document}
\title{Hybrid Beam Alignment for Multi-Path Channels: A Group Testing Viewpoint}
% \title{Beam Alignment with Multiple Beams: A Group Testing Viewpoint}
\author{Ozlem Yildiz\\
NYU Tandon School of Engineering,\\
Emails: zy2043@nyu.edu}

\maketitle

\begin{abstract}

The importance of the narrow beams increases with the usage of mmWave and tHz communication channels, which require beam alignment (BA) techniques to detect the channel clusters. For an uplink communication between single user equipment (UE) and a single base station (BS) which includes multiple channel clusters, analog and hybrid BA algorithms are derived by using the tools from the Group Testing literature. The proposed method outperformed the state-of-the-art. In this report, I focus on the literature review of our paper and summarize the main results.

\end{abstract}

\section{Introduction}

Next-generation wireless networks are operating in mmWave and THz frequencies due to the larger bandwidth availability and higher data rate demand \cite{mmWave-survey-nyu}. However, higher frequencies have some obstacles such as high path loss and shadowing, which require the use of directional beams.

Experimental results demonstrate that higher frequency channels consist of few spatial clusters \emph{i.e.} the channel is sparse \cite{akdeniz2014millimeter}. Hence, beam alignment (BA) techniques are necessary to localize the direction of these clusters. 

These techniques can be classified as \textit{interactive} or \textit{non-interactive}, and \textit{hybrid} or \textit{analog} BA. The first classification depends on the feedback delay of the scanning beams. If the BS is able to receive the result of the scanning beam before performing the next scanning beam, it is interactive; otherwise, it is non-interactive. The second classification depends on the number of Radio Frequency (RF) Chains, $N_{\rm RF}$. If $N_{\rm RF} = 1 $, it is analog BA, in which the BS can scan one beam at one time slot. If $N_{\rm RF} > 1  $, it is hybrid BA, where BS can scan $N_{\rm RF}$ scanning beams at one time slot.

In this report, I investigate the important literature for the paper in detail and discuss the results of the paper \cite{yildiz2021hybrid}. In the paper, we demonstrate a duality between hybrid interactive BA whose goal is to identify multiple paths and Group Testing (GT), which is a method to identify defective items from a set of items by pooling the items and testing them together \cite{aldridge2019group}. We propose algorithms importing tools from GT literature and demonstrate that proposed algorithms outperform the state-of-the-art results \cite{yildiz2021hybrid}.

\section{Literature Review}
In this section, I analyze the relevant literature for \cite{yildiz2021hybrid} in more detail. In Subsection \ref{multi}, I discuss the state-of-the-art analog BA result in \cite{aykin2019multi}. In Subsection \ref{gt}, I analyze the duality between GT and BA problem in \cite{suresh2019}. In Subsection \ref{freq}, I focus on GT application to the Internet of Things (IoT) with the parallel pooling tests. In Subsection \ref{hwang}, I explain the adaptive GT literature by Hwang \cite{hwang1972method} that we used for our hybrid BA methods. 

\subsection{Multi-Path Beam Alignment}
\label{multi}
Aykin \emph{et al.} \cite{aykin2019multi} analyze analog interactive BA to detect multiple channel clusters between a single UE and a single BS in a downlink scenario. They demonstrate a state-of-the-art multiple-path-detection method, called the multi-lobe beam search (MLBS) algorithm to detect the multiple paths. This method is optimized in noiseless settings and they test the algorithm in a noisy setting. 

MLBS is scanning $B$ angular intervals at each time slot to detect $M$ multiple clusters out of total $N$ angular intervals. The algorithm uses a binary decision tree to locate the angle of arrivals. However, to build the binary decision tree, a matrix of size ${N \choose M} \times {N \choose B}$ needs to be generated and the tree should be calculated. The proposed algorithm has high space complexity and the run time of the calculation of the binary decision tree is NP-hard. Note that the matrix generation and the binary decision tree building are offline calculations.

\subsection{Group Testing and Analog Beam Alignment}
\label{gt}

The novel correlation between GT and BA was studied by Suresh \emph{et al.} in \cite{suresh2019}. The authors analyze an analog non-interactive multi-path BA method for downlink communication scenario including a single UE and a single BS. They use the insights from the combinatorial GT literature \cite{du2000combinatorial}. They consider the noisy quantization scenario with an upper bound on the number of errors. The aim is to be resilient against the given maximum number of errors.

\subsection{Frequency Multiplexed Group Testing Strategy}
\label{freq}
GT has many applications in different fields such as medical testing, data science, cyber security, and IoT \cite{aldridge2019group}. Robin \emph{et al.} use GT methods to  IoT for a frequency multiplexed strategy. Therefore, they analyze GT problem with parallel tests. They consider Li's method \cite{li1962sequential} to parallelize the pooling tests due to the delay constraints. 

Li \cite{li1962sequential} considers multi-cycle GT method. In each cycle, there are multiple subgroups that are tested non-adaptively. Then, according to the test results of these multiple subgroups, the individuals are pooled together to build new subgroups for the next cycle. Therefore, this method is non-adaptive in each cycle but adaptive between cycles. 

According to the above discussion, it can be seen that the subgroups within the cycle can be tested parallel since there is no dependence on each other, and the authors in \cite{jyotishfrequency} exploit this feature of Li's method to parallelize the tests.

\subsection{Hwang's Generalized Binary Splitting}
\label{hwang}
In adaptive GT literature, Hwang's Generalized Binary Splitting \cite{hwang1972method} is an important result, since it's asymptotically optimal due to the number of tests, which is $O(d\log(N/d))$ for the sparse problems, a.k.a large $N/d$.

The breakthrough for adaptive GT is the discovery of the binary splitting algorithm, which is an optimal method to detect one defective item from a defective group by halving the group at every step. By using the binary splitting method, Hwang optimizes the parameters of the group size and determines the region where exhaustive search is more beneficial than the binary splitting algorithm with the knowledge of the upper bound on the number of defectives. The numerical comparisons in \cite{hwang1972method} demonstrate the improvement against the other adaptive GT strategies.

\section{Hybrid Beam Alignment for Multi-Path Channels: A Group Testing Viewpoint}

\subsection{Network Model and Beam Alignment} 
In our work, the communication is between a single BS and a single UE, where it consists of $M$ paths. At every slot of BA, UE transmits a BA packet, BS scans its angular region to find the direction of the path so the communication is uplink. The UE's transmission is omnidirectional while BS performs BA. Angle of arrivals (AoAs) of $M$ paths are i.i.d and uniform between $[0, 2\pi)$.

In this paper, BA is considered to be hybrid with $N_{\rm RF}$ RF chains and interactive. Therefore, BS scans $N_{\rm RF}$ beams at every time slot and the current scanning beam decision is dependent on the past scanning beams and their measurement results. Measurement results are binary, if AoA is detected, it is an acknowledgment (ACK); otherwise, it is negative ACK (NACK).

During BA, The BS uses fixed beamwidth $\omega$ to find the AoAs. The main goal of this paper is to localize $M$ AoAs with a minimum BA duration. The noise is not taken into consideration during the proposed algorithms' optimization, however, proposed algorithms are tested against the noise in the simulation section. 

\subsection{Proposed Algorithms and Results}

If data beamwidth which AoAs are detected is fixed $\omega$, there are $N = \frac{2 \pi}{\omega}$ angular intervals that BS can detect AoAs. Therefore, $N$ is the total number of items and $M$ is the upper bound on the total number of defectives since at most $M$ angular intervals can include AoAs. Therefore, if several angular intervals are pooled together to be tested (scanned), the duality with GT is clear. 

We propose to use Hwang's Generalized Binary Splitting \cite{hwang1972method} which has asymptotically optimal number of tests. The application of this GT method is suggested for analog BA. (Note that the BA problem is not in the asymptotic region due to hardware constraints). 

The analog GT-based BA (AGTBA) algorithm is compared against the state-of-the-art like MLBS and exhaustive search and it is demonstrated that BA duration is shorter, this justifies the application of Hwang's method \cite{hwang1972method}.

Later, our novel generalization of Hwang's Generalized Binary Splitting algorithm to the hybrid BA is discussed. Since Hwang's method is not designed to be parallelized, we suggest comparing three different extensions to the original algorithm for $N_{\rm RF} =2 $. 

The first extension is the divide and conquer method,  which divides the problem into $N_{\rm RF} =2 $ subgroups and solves them in parallel. The second extension is jointly solving the sub-problems by applying the binary splitting method when both subgroups result in ACK. Finally, the last extension similarly solves the problems jointly, however, it applies binary splitting for every ACK result. 

A comparison of the proposed algorithms suggests using the last described technique since it gives the best performance in terms of BA duration, improving upon AGTBA by a factor of two for $M=2$ and three for $M=4$. The noisy results also support the argument of the best performance.

\section{Conclusion}

In this report, I further investigated the most relevant literature and analysed them in more detail. Then, I discussed the results of the paper. In this paper, a novel hybrid BA algorithm based on GT method is discussed and OKsimulation results support the use of GT methods since the proposed methods outperform the state-of-the-art.

\bibliographystyle{IEEEtran}
\bibliography{ref}

\end{document}
